# Supplementary material for: The Paths to Choreography Extraction
Source: arXiv:1610.10050 source file (2017-02-20)
Supplement: Supplementary file 1 [file appendix.tex]

\subsection*{Full semantics of SP}

The full semantics of SP is given in Figure~\ref{fig:sp_semantics_full}.
\begin{figure}[t]
% {\footnotesize
\begin{eqnarray*}
&\infer[\rname{S}{Com}]
{
	\actor{\pid p}{}{\asend{\pid q}{e};B_1}
	\ \parp\ 
	\actor{\pid q}{}{\arecv{\pid p};B_2},\ \sigma
	\ \lto{\com{\pid p.v}{\pid q}} \ 
	\actor{\pid p}{}{B_1}
	\ \parp\ 
	\actor{\pid q}{}{B_2},\ \sigma[\pid q \mapsto v]
}
{
	e[\sigma(\pid p)/\pcont] \eval v
}
\\[1ex]
& \infer[\rname{S}{Ctx}]
{
\actor{\pid p}{}{\rec{X}{B_2}{B_1}}
\ \parp\ 
N,\ \sigma
\quad \lto\lambda \quad
\actor{\pid p}{}{\rec{X}{B_2}{B'_1}}
\ \parp\ 
N', \ \sigma'
}{
\actor{\pid p}{}{{B_1}}
\ \parp\ 
N,\ \sigma
\quad \lto\lambda \quad
\actor{\pid p}{}{{B'_1}}
\ \parp\ 
N', \ \sigma'
}
\\[1ex]
&\infer[\rname{S}{Sel}]
{
	\actor{\pid p}{}{\asel{\pid q}{l_j};B}
	\ \parp\ 
	\actor{\pid q}{}{\abranch{\pid p}{\{ l_i : B_i\}_{i\in I}}},\ \sigma
	\ \lto{\gensel} \
	\actor{\pid p}{}{B}
	\ \parp\ 
	\actor{\pid q}{}{B_j},\ \sigma
}
{j \in I}
\\[1ex]
&\infer[\rname{S}{Then}]
{
	\actor{\pid p}{}{\cond{\eqcom{\pcont}{\pid q}}{B_1}{B_2}}
	\ \parp\ 
	\actor{\pid q}{}{\asend{\pid p}{e};B'},\ \sigma
	\ \lto{\condlbl{\pid p}{\pid q}{\m{then}}} \ 
	\actor{\pid p}{}{B_1}
	\ \parp \ 
	\actor{\pid q}{}{B'},\ \sigma
}
{
	e[\sigma(\pid q)/\pcont]\eval \sigma(\pid p)
}
\\[1ex]
&\infer[\rname{S}{Else}]
{
	\actor{\pid p}{}{\cond{\eqcom{\pcont}{\pid q}}{B_1}{B_2}}
	\ \parp\ 
	\actor{\pid q}{}{\asend{\pid p}{e};B'},\ \sigma
	\ \lto{\condlbl{\pid p}{\pid q}{\m{else}}} \ 
	\actor{\pid p}{}{B_2}
	\ \parp \ 
	\actor{\pid q}{}{B'},\ \sigma
}
{
	e[\sigma(\pid q)/\pcont]\not \eval \sigma(\pid p)
}
\\[1ex]
&
\infer[\rname{S}{Par}]
{
	N \parp M,\ \sigma \quad \lto\lambda \quad N' \parp M,\ \sigma'
}
{
	N,\ \sigma \ \lto\lambda\  N',\ \sigma'
}
\qquad
\infer[\rname{S}{Struct}]
{
	N,\sigma \quad \lto\lambda \quad N', \sigma'
}
{
	N \precongr M & M,\sigma\ \lto\lambda \ M',\sigma' & M' \precongr N'
}
\end{eqnarray*}
% }
\caption{Stateful Processes, Semantics.}
\label{fig:sp_semantics_full}
\end{figure}

\subsection*{EndPoint Projection}
EPP is inductively defined by the rules in Figure~\ref{fig:epp}.
\begin{figure}[t]
\begin{align*}
& \epp{C,\sigma}{}  =
\prod_{\pid p \in \pn(C)} \actor{\pid p}{\sigma(\pid p)}{\epp{C}{\pid p}}
\\[1ex]
\hline
\\
&
\epp{\gencom;C}{\pid r} =
	\begin{cases}
		\asend{\pid q}{e};\epp{C}{\pid r} & \text{if } \pid r = \pid p \\
		\arecv{\pid p};\epp{C}{\pid r} & \text{if } \pid r = \pid q \\
		\epp{C}{\pid r} & \mbox{o.w.}
	\end{cases}
\quad\qquad
\epp{\gensel;C}{\pid r} =
	\begin{cases}
		\asel{\pid q}{l};\epp{C}{\pid r} & \text{if } \pid r = \pid p \\
		\abranch{\pid p}{\{ l : \epp{C}{\pid r} \}} & \text{if } \pid r = \pid q \\
		\epp{C}{\pid r} & \mbox{o.w.}
	\end{cases}
\\[1ex]
&\epp{\gencond}{\pid r} =
	\begin{cases}
		\cond{\eqcom{\pcont}{\pid q}}{\epp{C_1}{\pid r}}{\epp{C_2}{\pid r}} & \text{if } \pid r = \pid p \\
		\asend{\pid p}{\pcont}; ( \epp{C_1}{\pid r} \merge \epp{C_2}{\pid r} ) & \text{if } \pid r = \pid q \\
		\epp{C_1}{\pid r} \merge \epp{C_2}{\pid r} & \mbox{o.w.}
	\end{cases}
\qquad\quad
\epp{\nil}{\pid r} = \nil
\\[1ex]
&
	\epp{\rec{X^{\pids p}}{C_2}{C_1}}{\pid r} =
		\begin{cases}
			\rec{X}{\epp{C_2}{\pid r}}{\epp{C_1}{\pid r}}
			& \text{if } \pid r \in \pids p \\
			\epp{C_1}{\pid r} & \mbox{o.w.}
		\end{cases}
\quad\qquad
\epp{X^{\pids p}}{\pid r} =
	\begin{cases}
		\call{X}
		& \text{if } \pid r \in \pids p \\
		\nil & \mbox{o.w.}
	\end{cases}
\end{align*}
\caption{Core Choreographies, EndPoint Projection (EPP).}
\label{fig:epp}
\end{figure}
EPP produces a parallel composition with one process for each one process name in the original choreography.
The rules for projecting process behaviors follow the intuition of projecting the local action performed by the 
process of interest.
The rules for projecting recursive definitions and calls assume that
procedure names have been annotated with the process names appearing
inside the body of the procedure, in order to avoid projecting
unnecessary procedure code (see~\cite{CM16b}).
The rule for projecting a conditional uses the partial
merging operator $\merge$ to merge the possible behaviors of a process that does not know
which branch will be chosen. Merging is a homomorphic binary operator; for
all terms but branchings it requires isomorphism, e.g.:
$\asend{\pid q}{e};B \merge \asend{\pid q}{e};B' = \asend{\pid q}{e};(B \merge B')$.
Branching terms can have unmergeable continuations, as long as they are
guarded by distinct labels. In this case, merge returns a larger branching
including all options (merging branches with the same label):
\begin{multline*}
  \abranch{\pid p}{\{l_i:B_i\}_{i\in J}} \merge
  \abranch{\pid p}{\{l_i:B'_i\}_{i\in K}} =\\
  \abranch{\pid p}{\left(\{l_i:(B_i \merge B'_i)\}_{i\in J\cap K}\cup\{l_i:B_i\}_{i\in J \setminus 
K}\cup\{l_i:B'_i\}_{i\in K \setminus J}\right)}
\end{multline*}

\subsection*{Proofs of results on extraction (finite case)}

\begin{proof}[Lemma~\ref{lem:sound-fin}]
  By definition, $\rwto$ has the diamond property,
  and all the possible diamonds correspond exactly to rules in the definition of the structural precongruence relation for CC.
  The thesis then follows by induction on the number of rewriting steps in $N\rwto^\ast C_1$.
\end{proof}

\begin{proof}[Theorem~\ref{thm:correct}]
  Straightforward by structural induction on $C$.
\end{proof}

\begin{remark}
  The extracted choreography can be exponential in the size of the original network.
  Consider the family of networks $\mathcal N_n$ defined as follows.
  \[
  \mathcal N_n = \prod_{i=1}^n
  \left(
  \actor{\pid p_{2i-1}}{}{\cond{\eqcom{\pcont}{\pid p_{2i}}}{\nil}{\nil}}
  \parp\actor{\pid p_{2i}}{}{\bsend{\pid p_{2i-1}}{e}}
  \right)
  \]
  $\mathcal N_n$ contains exactly $2n$ actions, of which half are conditionals and half are message sends.
  A straightforward induction proof establishes that every choreography $C$ such that
  $\extract{\mathcal N_n}\rwto^\ast C$ contains $2^n-1$ conditionals (and no other actions).
\end{remark}

\subsection*{Encoding top-level definitions in CC}
We show how to encode top-level definitions in the original syntax of CC.
We illustrate the exponential growth by means of a choreography with two mutually recursive definitions:
$\langle\{X=C_X,Y=C_Y\},C\rangle$ where both $C_X$, $C_Y$ and $C$ contain calls to $X$ and $Y$.
If we try to define it as a choreography of the form $\genrec$, then both $C_1$ and $C_2$ must be able to
invoke $Y$, which means we have to duplicate the definition of $Y$, obtaining
\[
\rec{X}{\left(\rec{Y}{C_Y}{C_X}\right)}{\left(\rec{Y'}{C_Y[Y'/Y]}{C[Y'/Y]}\right)}
\]
and the terms in parentheses correspond to the choreographies $\langle\{Y=C_Y\},C_X\rangle$ and
$\langle\{Y=C_Y\},C\rangle$ (where they are allowed to use $X$).

In general, we can therefore encode procedure definitions at the top by means of an operator
$\ohgod{\mathcal D,C}$ defined as
\begin{align*}
  \ohgod{\emptyset,C} &= C \\
  \ohgod{\{X=C_X\}\cup\mathcal D,C\}}
  &= \rec{X}{\ohgod{\mathcal D,C_X}}{\ohgod{\mathcal D,C}}
\end{align*}
where we rely on $\alpha$-renaming to obtain different names for the procedures defined in the two recursive
calls to $\ohgod\cdot$.
%\todo{say something about using CC notation when easy}

\begin{theorem}
  The choreographies $\langle\mathcal D,C\rangle$ and $\ohgod{\mathcal D,C}$ are behaviorally equivalent.
\end{theorem}

\subsection*{Proofs of results on extraction (general case)}

\begin{proof}[Theorem~\ref{thm:aes-good}]
  We describe an algorithm to find a valid SEG in the AES, if it exists.
  To make it clearer, we first describe how one (possibly invalid) SEG could be found.
  Start with the node representing the initial network and move along edges in the graph, noting that if an
  edge labeled $\lto{\condlbl{\pid p}{\pid q}{\m{then}}}$ is chosen, then the path containing the
  corresponding $\m{else}$ action must also be taken (and reciprocally).
  We keep exploring the graph until all paths explored end or loop into nodes already explored.
  Given the method of construction, we can view this as a tree with loops back to earlier nodes.
  This construction will give us one SEG.

  To find a \emph{valid} SEG, we backtrack over all the nodes where there were alternative path continuations.
  We enumerate nodes consecutively as we explore them, so if their number is different from the initial dummy
  value, we have found a loop.
  From such a node where we just discovered that a loop started, we can traverse the loop again by going
  towards the node with larger (initialized) number whenever there is a choice, and check for the existence of
  an all-white node somewhere on the loop.
  If found, we proceed recursively with the latest unexplored branch.
  Otherwise, we backtrack, choosing the most recent unexplored choice.

  If there are no more possible unexplored alternatives, then one of the processes in the node where the loop
  started is deadlocked in all subsequent states, contradicting the hypothesis.
\end{proof}

\begin{proof}[Theorem~\ref{thm:oc-ac-ap}, sketch]
  Let $N$ be a network and $C$ be a choreography extracted from $N$.
  Define a relation $\mathcal R\subseteq \mathcal C\times\mathcal N$, where
  $\mathcal C=\{C'\mid C\to^\ast C'\}$ and $\mathcal N=\{N'\mid N\to^\ast N'\}$, as follows:
  $C'\mathcal R N'$ if $C\to^\ast C'$ and $N\to^\ast N'$ with the same sequence of actions.
  We prove that $\mathcal R$ is a bisimulation by induction on the length of this sequence.

  If the sequence is empty and $C\to C''$, then clearly $N\to N''$ with the same action, since $C$ is defined
  by choosing an action that $N$ can make.
  If $N\to N''$, there are two cases; the interesting one is when the action taken is not the same as
  specified at the top of $C$.
  Note that the processes involved are not able to participate in any other reductions, so the action remains
  enabled in all execution paths of $N$, in particular in that taken by $C$, and is swappable with every
  action in $C$.
  Then we simply need to show that $C$ eventually takes this action, which is guaranteed by the fairness
  conditions imposed in Definition~\ref{defn:valid-seg}.

  If this sequence is not empty, the proof for the case when $C'$ makes a move remains the same.
  For the case when $N'$ makes a move, we can make a similar argument by considering the actions from $N$ to
  $N'$ that occur at the top level in $C$, which are necessarily swappable with the remaining ones; so $C$ can
  reduce to a choreography $C^\ast$, which can execute the action executed by $N'$ (as in the base case) and
  then the remaining actions in the reduction from $N$ to $N'$ to $C''$.
  Again by swapping, also $C'\to C''$.
\end{proof}

\begin{proof}[Lemma~\ref{lem:size-aes}]
Let $N$ be a network with $p$ processes of sizes $n_1$ through $n_p$, where the size of a process is the
number of nodes in an abstract syntax tree representing the syntactical term.
We let $n=\sum_{i=1}^p n_i$ denote the size of $N$.

Since recursive definitions are unfolded only when they occur at the top of a behavior, a process of size
$n_i$ can give rise to at most $n_i$ different terms when all possible reductions are considered.
Thus, $N$ can reduce to at most $\prod_{i=1}^p n_i$ different terms.
Since the reductions give rise to the edges in the graph,
this is also an upper bound on the number of edges,
so the graph is sparse.
By the AM-GM inequality,
$\prod_{i=1}^p n_i$ is maximized when all the $n_i$ are equal,
where it evaluates to $\left(\frac{n}{p}\right)^p$.
% %% When creating the AES graph, we unfold recursive definitions only
% %% when necessary, i.e., at the point where an action has to come from
% %% a variable (a procedure call). Thus, a process of size $n_i$ can give
% %% rise to $n_i$ different terms when all possible reductions are
% %% considered recursively. All in all, $\prod_{i=1}^p n_i$ is then an upper bound on
% %% the number of terms the network as a whole can reduce to.
% %% The graph is sparse.
% %% The $i$th process has only $n_i$ possible actions, so there cannot be
% %% a total of more than $\prod_{i=1}^p n_i$ reductions; fewer if some
% %% actions are combined in a communication.
% %% By the AM-GM inequality, this is maximized when all the $n_i$ are equal,
% %% giving $\left(\frac{n}{p}\right)^p$ as an upper bound.
% %%
% %% Taking the annotations into account, we observe that for each process,
% %% either all procedure calls are marked with $\circ$, or they are all
% %% marked by $\bullet$, so there are $2^p$ combinations for each term,
% %% giving a total upper bound of
% %% $2^p(\frac{n}{p})^p=(\frac{2n}{p})^p$ different nodes in the graph.
% %% %
% %% It is easy to show that this expression attains its maximum
% %% when $p=\frac{2n}{e}$,
% %% where $e$ is Euler's number,
% %% giving the upper bound of $e^{\frac{2n}{e}}$ nodes in the AES graph.
% 
We now consider annotations.
We observe that all procedure calls in the same process must be marked with the same token, so there are at
most $2^p$ annotations for each network, giving a total upper bound of
$2^p(\frac{n}{p})^p=(\frac{2n}{p})^p$ different nodes in the AES.
This expression attains its maximum when $p=\frac{2n}{e}$, where $e$ is Euler's
number, giving the upper bound of $e^{\frac{2n}{e}}$ nodes in the AES graph.\qed
\end{proof}

\begin{proof}[Theorem~\ref{thm:extract-complex}]
Constructing the graph can be done iteratively by maintaining a set of unexplored nodes.
Whenever an unexplored node is examined, the possible reductions lead to new terms; by keeping all created
nodes in a search structure, we can check if the node already exists (and get a reference to it) in
logarithmic time in the number of nodes (which is $O(n)$) and linear time in the size of the term (which is
also logarithmic in the size of the graph).
Thus, the AES can be constructed with overall complexity $O(n e^{\frac{2n}{e}})$.

To extract a valid SEG from the AES, we perform a graph traversal, which is linear in the size of the
graph.
There is the one complication, however: checking that loops contain an all-white node.
Rechecking the entire loop could potentially move the overall complexity to factorial time; we explain how to
handle this without increasing the asymptotic time complexity.
Recall from the proof of Theorem~\ref{thm:aes-good} that we stop our search and start backtracking when we
discover a loop; we thus conceptually have a path from the start node to our current node at all times, and
the path behaves in a stack-like manner.
We introduce an explicit stack as an auxiliary data structure.
Each node on the current path has a pointer to its entry on the stack.
An item on the stack contains a boolean stating if its corresponding node is all-white and a counter of how
many white nodes can be found further down on the stack.
This information can easily be maintained in constant time as we push and pop elements in connection with
running the backtracking algorithm.
When we encounter a loop, we follow the pointer to the node's associated stack item and check the counter,
$c$.
The loop just found has at least one white node if and only if the counter of the top item on the stack is
strictly greater than $c$.
\end{proof}
